# Supplementary material for: Dynamic Hypergames for Synthesis of Deceptive Strategies with Temporal Logic Objectives
Source: arXiv:2007.15726 source file (2020-07-30)
Supplement: Supplementary file 1 [file appendix.tex]

% \paragraph{Offline trajectories}
% \allowdisplaybreaks
% With a slight abuse of notation, we denote the projection of $h$ onto the set of actions $A_1$ as $h \downharpoonright_{A_1}$.
% \begin{itemize}
%     \item The observed trajectory induced $h^R$ by the random policy $\pi_2^R$:
%         \begin{align*}
%             h^R \downharpoonright_S = & [(2, 4), (1, 4), (0, 4), (1, 4), (2, 4), (3, 4), (3, 4), (4, 4), (4, 4), (4, 4), (4, 3), (4, 2), (4, 1), (4, 0)] \\
%             h^R \downharpoonright_{A_1} = & [(-1, 0), (-1, 0), (1, 0), (1, 0), (1, 0), (1, 0), (1, 0), (1, 0), (1, 0), (1, 0), (0, -1), (0, -1), (0, -1)]
%         \end{align*}
%     The augmented state-action sequence $\tilde h^R$ transformed from the history $h^R$:
%         \begin{align*}
%             \tilde h^R\downharpoonright_{\tilde V} = 
%             & [((('g1', (((2, 4), (2, 0)),)), 1), 0), ((('g1', (((2, 4), (2, 0)), ((-1, 0), (3, 4)), ((1, 4), (3, 4)))), 1), 0),
%             \\ & ((('g3', (((1, 4), (3, 4)), ((-1, 0), (0, 2)), ((0, 4), (0, 2)))), 2), 0), 
%             \\ & ((('g3', (((0, 4), (0, 2)), ((1, 0), (2, 0)), ((1, 4), (2, 0)))), 2), 0), 
%             \\ & ((('g3', (((1, 4), (2, 0)), ((1, 0), (2, 0)), ((2, 4), (2, 0)))), 2), 0), 
%             \\ & ((('g2', (((2, 4), (2, 0)), ((1, 0), (0, 2)), ((3, 4), (0, 2)))), 2), 0), 
%             \\ & ((('g2', (((3, 4), (0, 2)), ((1, 0), (2, 0)), ((3, 4), (2, 0)))), 2), 0), 
%             \\ & ((('g2', (((3, 4), (2, 0)), ((1, 0), (0, 2)), ((4, 4), (0, 2)))), 2), 0), 
%             \\ & ((('g2', (((4, 4), (0, 2)), ((1, 0), (0, 2)), ((4, 4), (0, 2)))), 2), 0), 
%             \\ & ((('g2', (((4, 4), (0, 2)), ((1, 0), (0, 2)), ((4, 4), (0, 2)))), 2), 0), 
%             \\ & ((('g2', (((4, 4), (0, 2)), ((1, 0), (0, 2)), ((4, 3), (0, 2)))), 2), 0), 
%             \\ & ((('g2', (((4, 3), (0, 2)), ((0, -1), (3, 4)), ((4, 2), (3, 4)))), 2), 0), 
%             \\ & ((('g1', (((4, 2), (3, 4)), ((0, -1), (2, 0)), ((4, 1), (2, 0)))), 2), 0), 
%             \\ & ((('g1', (((4, 1), (2, 0)), ((0, -1), (2, 0)), ((4, 0), (2, 0)))), 0), 0)]
%         \end{align*}
%     The observed trajectory induced $h^B$ by the policy $\pi_2^{B, 2}(x)$, where $x$ is from the inference function $\eta$:
%         \begin{align*}
%             h^B \downharpoonright_S = & [(2, 4), (1, 4), (0, 4), (1, 4), (1, 3), (0, 3), (1, 3), (1, 4), (2, 4), (3, 4), (4, 4), (4, 4), (4, 4), (4, 4), (4, 3), (4, 2), (4, 1), \\
%             & (4, 2), (4, 1), (4, 1), (4, 0)] \\
%             h^B \downharpoonright_{A_1} = & [(-1, 0), (-1, 0), (1, 0), (1, 0), (0, 1), (0, 1), (0, 1), (1, 0), (1, 0), (1, 0), (1, 0), (1, 0), (1, 0), (1, 0), (0, -1), (0, -1), \\
%             & (-1, 0), (0, -1), (0, 1), (0, -1)]
%         \end{align*}
%     The augmented state-action sequence $\tilde h^B$ transformed from the history $h^B$:
%         \begin{align*}
%             \tilde h^B\downharpoonright_{\tilde V} = 
%             & [((('g1', (((2, 4), (2, 0)),)), 1), 0), ((('g1', (((2, 4), (2, 0)), ((-1, 0), (3, 4)), ((1, 4), (3, 4)))), 1), 0),
%             \\ & ((('g3', (((1, 4), (3, 4)), ((-1, 0), (0, 2)), ((0, 4), (0, 2)))), 2), 0), 
%             \\ & ((('g3', (((0, 4), (0, 2)), ((1, 0), (0, 2)), ((1, 4), (0, 2)))), 2), 0), 
%             \\ & ((('g3', (((1, 4), (0, 2)), ((1, 0), (2, 0)), ((1, 3), (2, 0)))), 2), 0), 
%             \\ & ((('g2', (((1, 3), (2, 0)), ((0, 1), (2, 0)), ((0, 3), (2, 0)))), 2), 0), 
%             \\ & ((('g2', (((0, 3), (2, 0)), ((0, 1), (3, 4)), ((1, 3), (3, 4)))), 2), 0), 
%             \\ & ((('g3', (((1, 3), (3, 4)), ((0, 1), (3, 4)), ((1, 4), (3, 4)))), 2), 0), 
%             \\ & ((('g3', (((1, 4), (3, 4)), ((1, 0), (2, 0)), ((2, 4), (2, 0)))), 2), 0), 
%             \\ & ((('g2', (((2, 4), (2, 0)), ((1, 0), (2, 0)), ((3, 4), (2, 0)))), 2), 0), 
%             \\ & ((('g2', (((3, 4), (2, 0)), ((1, 0), (3, 4)), ((4, 4), (3, 4)))), 2), 0), 
%             \\ & ((('g2', (((4, 4), (3, 4)), ((1, 0), (3, 4)), ((4, 4), (3, 4)))), 2), 0), 
%             \\ & ((('g2', (((4, 4), (3, 4)), ((1, 0), (3, 4)), ((4, 4), (3, 4)))), 2), 0), 
%             \\ & ((('g2', (((4, 4), (3, 4)), ((1, 0), (3, 4)), ((4, 4), (3, 4)))), 2), 0), 
%             \\ & ((('g2', (((4, 4), (3, 4)), ((1, 0), (3, 4)), ((4, 3), (3, 4)))), 2), 0), 
%             \\ & ((('g2', (((4, 3), (3, 4)), ((0, -1), (3, 4)), ((4, 2), (3, 4)))), 2), 0), 
%             \\ & ((('g1', (((4, 2), (3, 4)), ((0, -1), (3, 4)), ((4, 1), (3, 4)))), 2), 0), 
%             \\ & ((('g1', (((4, 1), (3, 4)), ((-1, 0), (0, 2)), ((4, 2), (0, 2)))), 2), 0), 
%             \\ & ((('g3', (((4, 2), (0, 2)), ((0, -1), (0, 2)), ((4, 1), (0, 2)))), 2), 0), 
%             \\ & ((('g1', (((4, 1), (0, 2)), ((0, 1), (2, 0)), ((4, 1), (2, 0)))), 2), 0), 
%             \\ & ((('g2', (((4, 1), (2, 0)), ((0, -1), (0, 2)), ((4, 0), (0, 2)))), 0), 0)]
%         \end{align*}
% \end{itemize}


% \paragraph{Online trajectories}
% The online trajectory $h^O$ induced by the random policy $\pi_2^R$:
%         \begin{align*}
%             h^O \downharpoonright_S = & [(2, 4), (1, 4), (1, 4), (0, 4)]\\
%             h^O \downharpoonright_{A_1} = & [(3, 4), (0, 2), (0, 2)]
%         \end{align*}
%     The augmented state-action sequence $\tilde h^O$ transformed from the history $h^O$:
%         \begin{align*}
%             \tilde h^O\downharpoonright_{\tilde V} = 
%             & [((('g1', (((2, 4), (2, 0)),)), 1), 0), ((('g1', (((2, 4), (2, 0)), ((-1, 0), (3, 4)), ((1, 4), (3, 4)))), 1), 0),
%             \\ & ((('g3', (((1, 4), (3, 4)), ((-1, 0), (0, 2)), ((1, 4), (0, 2)))), 1), 0), 
%             \\ & ((('g3', (((1, 4), (0, 2)), ((-1, 0), (0, 2)), ((0, 4), (0, 2)))), 2), 0)]
%         \end{align*}
