# Supplementary material for: Dynamic Hypergames for Synthesis of Deceptive Strategies with Temporal Logic Objectives
Source: arXiv:2007.15726 source file (2020-07-30)
Supplement: Supplementary file 2 [file appendix.tex]

\section{Pseudo Code}~\label{sec:pseudo_code}
\begin{algorithm}[!htb]
\begin{algorithmic}[1]
\renewcommand{\algorithmicrequire}{\textbf{Input:}}
\renewcommand{\algorithmicensure}{\textbf{Output:}}
\REQUIRE{The current history $h_0$}
\ENSURE{Best action $a$}
\STATE{create rood node $v_0$ with history $h_0$}
\WHILE{within computational budget}
\STATE{$v_l \leftarrow TREEPOLICY(v_0)$}
\STATE{$\Delta \leftarrow DEAFAULTPOLICY(h(v_l))$}
\STATE{$BACKUP(v_l, \Delta)$}
\ENDWHILE
\RETURN{$a(BESTCHILD(v_0))$}
\end{algorithmic}
\caption{MCTP search}
\label{alg:mcts}
\end{algorithm}

\begin{algorithm}[!htb]
\begin{algorithmic}[1]
\renewcommand{\algorithmicrequire}{\textbf{Input:}}
\renewcommand{\algorithmicensure}{\textbf{Output:}}
\REQUIRE{The current node $v$}
\ENSURE{The the most urgent expandable node $v$, or a nonterminal node $v$ and has unvisited}
\WHILE{$v$ is non-terminal}
\IF{$v$ not fully expanded}
\RETURN{$EXPAND(v)$}
\ELSE{\STATE{$v \leftarrow BESTCHILD(v, Cp)$}}
\ENDIF
\ENDWHILE
\RETURN{$v$}
\end{algorithmic}
\caption{TREEPOLICY}
\label{alg:tree_policy}
\end{algorithm}

\begin{algorithm}[!htb]
\begin{algorithmic}[1]
\renewcommand{\algorithmicrequire}{\textbf{Input:}}
\renewcommand{\algorithmicensure}{\textbf{Output:}}
\REQUIRE{$v$}
\ENSURE{$v'$}
\STATE{$a \in untried actions from A(h(v))$}
\STATE{add a new child $v'$ to $v$}
    \STATE{with $h(v') = f(h(v),a)$ and $a(v') = a$}
\RETURN{v'}
\end{algorithmic}
\caption{EXPAND}
\label{alg:expand}
\end{algorithm}


\begin{algorithm}[!htb]
\begin{algorithmic}[1]
\renewcommand{\algorithmicrequire}{\textbf{Input:}}
\renewcommand{\algorithmicensure}{\textbf{Output:}}
\REQUIRE{$v,c$}
\ENSURE{$v'$}
\RETURN{$\arg \max_{v' \in children of v} \frac{Q(v')}{N(v')} + c \sqrt{\frac{2 \ln{N(v)}}{N(v')}}$}
\end{algorithmic}
\caption{BESTCHILD}
\label{alg:best_child}
\end{algorithm}

\begin{algorithm}[!htb]
\begin{algorithmic}[1]
\renewcommand{\algorithmicrequire}{\textbf{Input:}}
\renewcommand{\algorithmicensure}{\textbf{Output:}}
\REQUIRE{$v, r$}
\ENSURE{$v$}
\WHILE{$v$ is not null}
\STATE{$N(v) \leftarrow N(v) + 1$}
\STATE{$Q(v) \leftarrow Q(v) + r(v)$}
\STATE{$v \leftarrow$ parent of $v$}
\ENDWHILE
\end{algorithmic}
\caption{BACKUP}
\label{alg:backup}
\end{algorithm}
